# Supplementary material for: High molecular gas content and star formation rates in local galaxies that host quasars, outflows and jets
Source: arXiv:2007.10351 ancillary file (2020-07-20)
Supplement: Supplementary file 1 [file jarvis20_CO_paper_supplement.pdf]

MNRAS 000, 1–1 (0000) Preprint 18 July 2020 Compiled using MNRAS LaTeX style file v3.0

# Supplement to Appendix A

This document contains corner plots showing the posterior probability distributions of each of the parameters for each source (Fig. A1-A12).

This paper has been typeset from a TeX/LaTeX file prepared by the author.

© 0000 The Authors

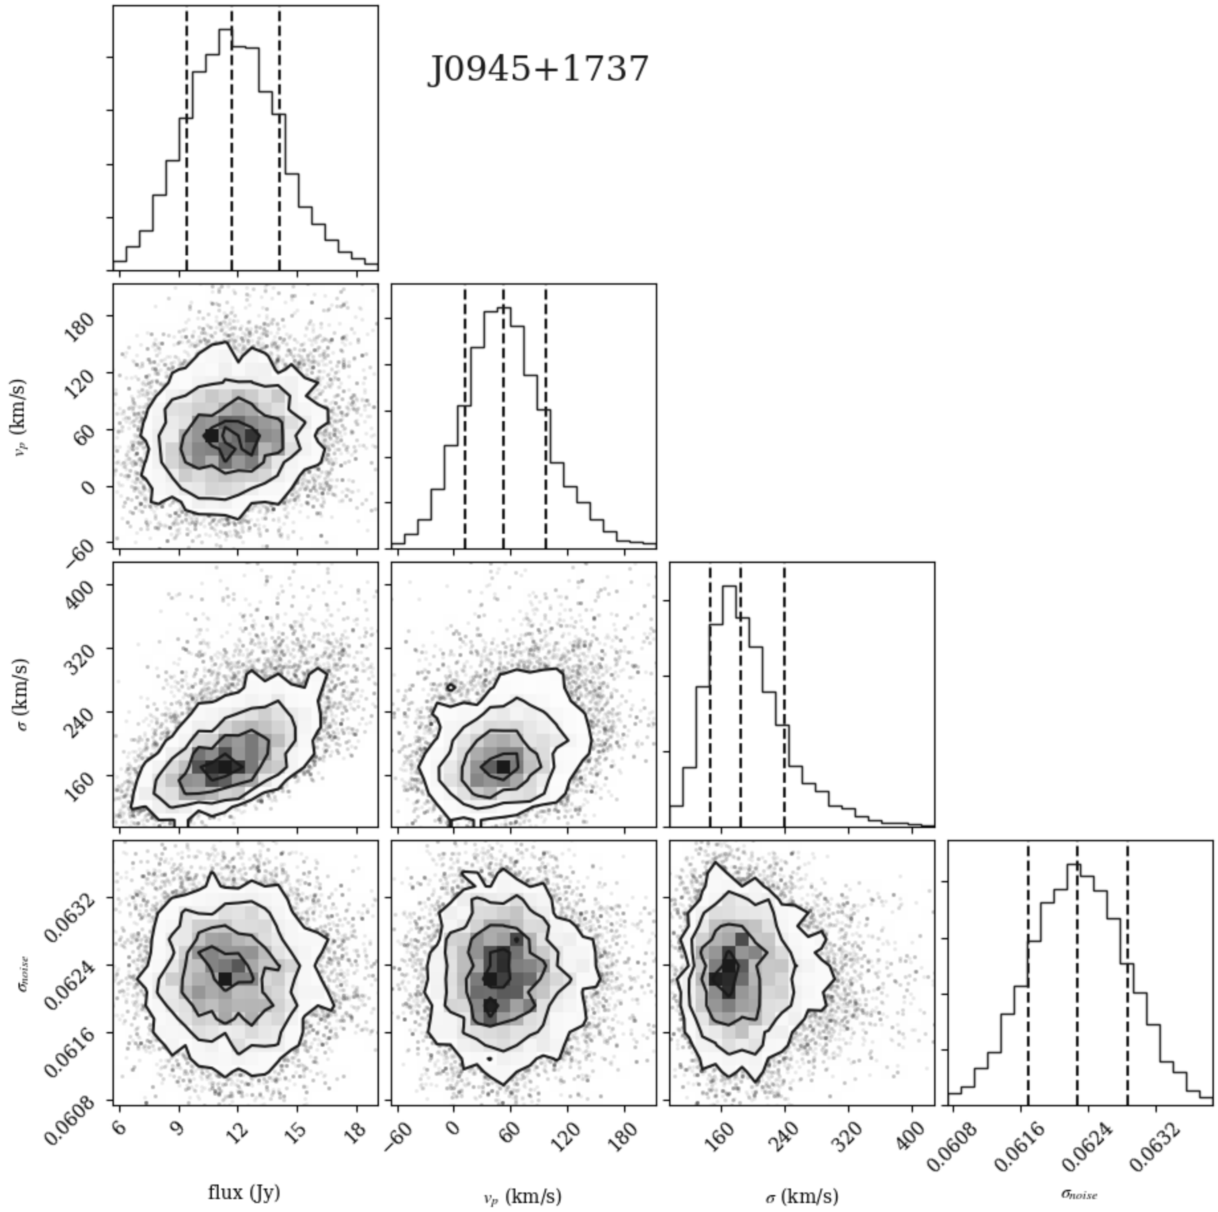


**Figure A1.** Corner plot showing all the one and two dimensional projections of the posterior probability distributions of our parameters for the APEX CO(2–1) data for J0945+1737. The parameters are: the emission line flux (f), peak velocity ($v_p$), standard deviation ($\sigma$; line width) and the standard deviation of the noise ($\sigma_N$). The limits on each axis are the 0.3 and 99.7th percentiles of that parameter. The 16, 50, 84th percentiles are shown as dashed black lines in the one dimensional posterior distribution for each parameter (ie. the value and errors given in Table 3).

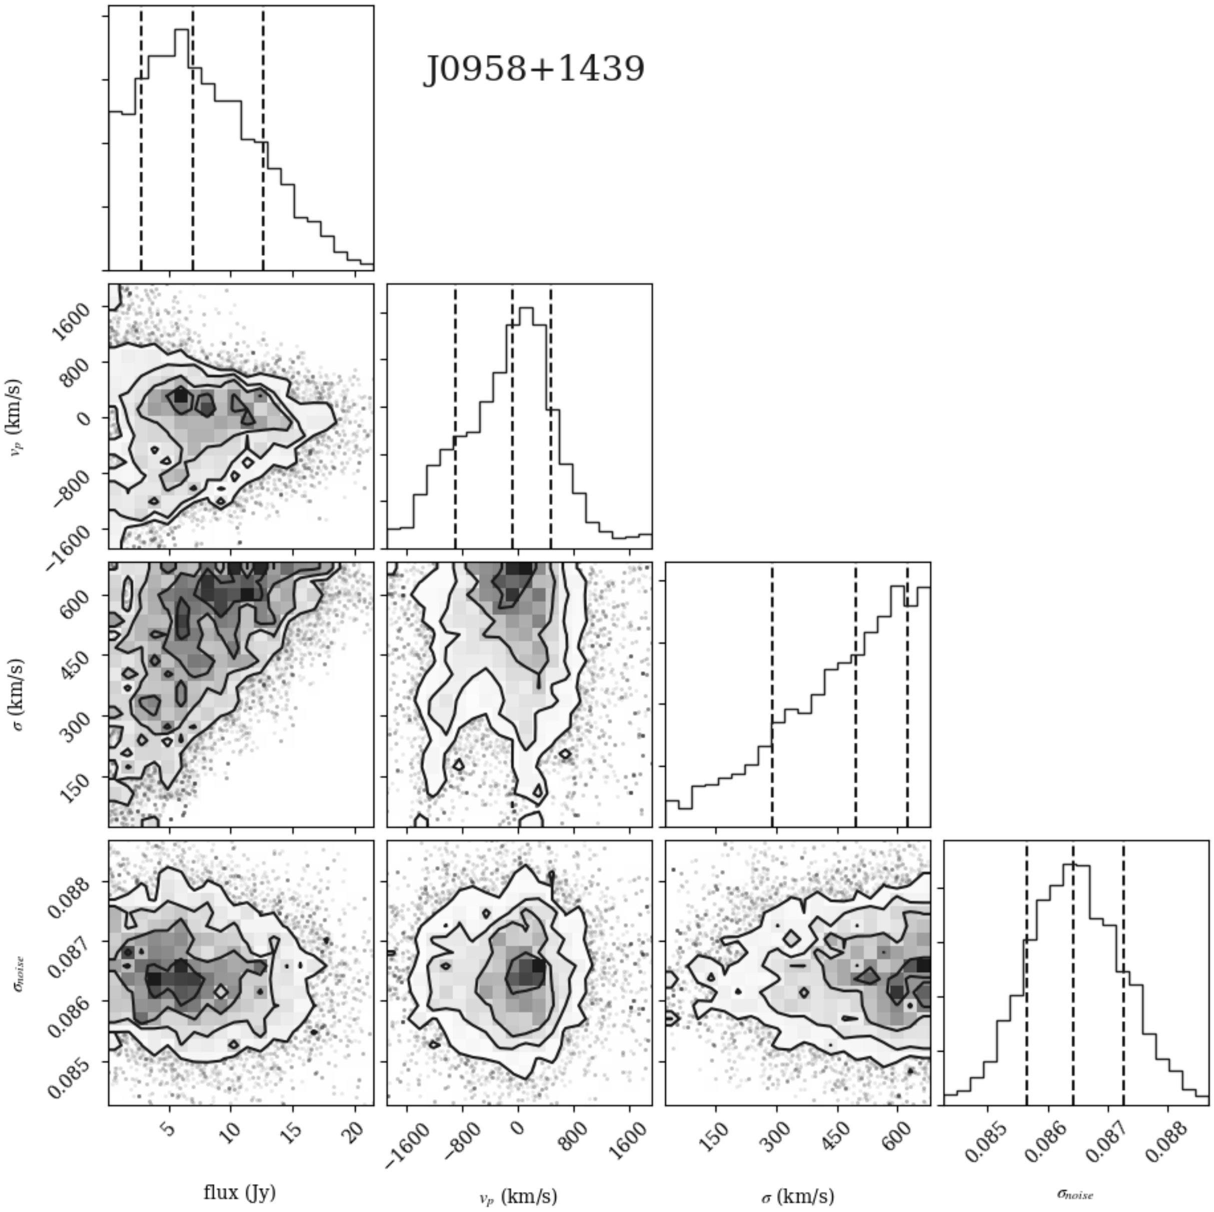


**Figure A2.** Same as Fig. A1 but for J0958+1439. The posteriors clearly show that the maximum allowed $\sigma$ is preferred, with the one dimensional posterior distribution for $\sigma$ rising steadily to the maximum value. This supports our identification of this data as a non-detection. The limit of the flux axes is the 99.7th percentile which is what we use as the upper limit of the CO(2–1) flux for our analysis.

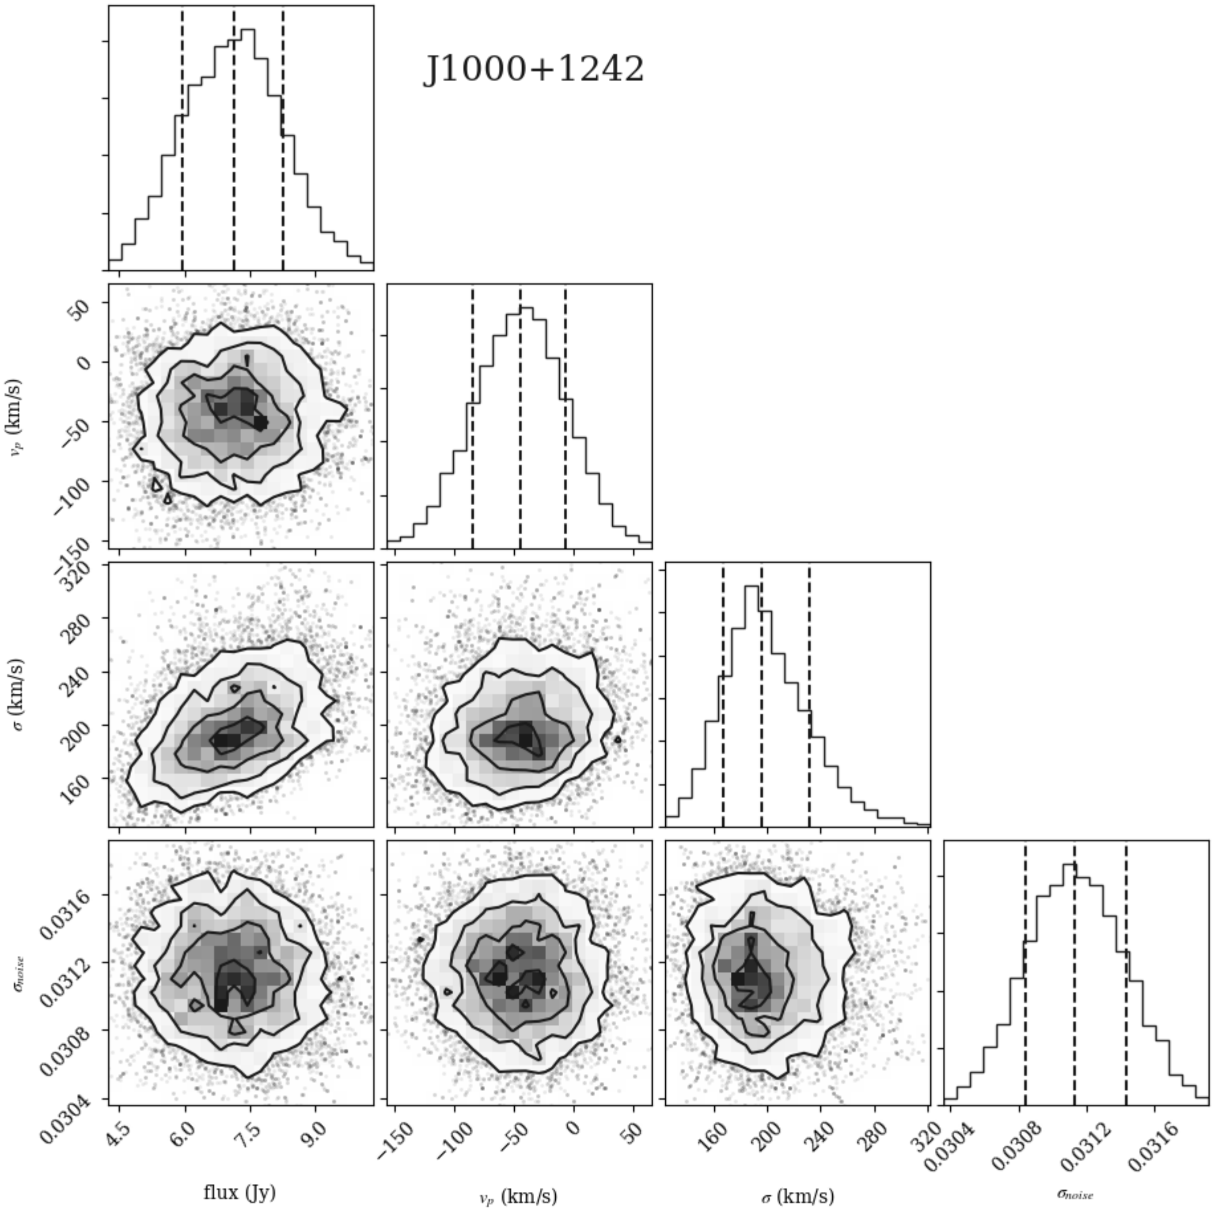


**Figure A3.** Same as Fig. A1 but for J1000+1242.

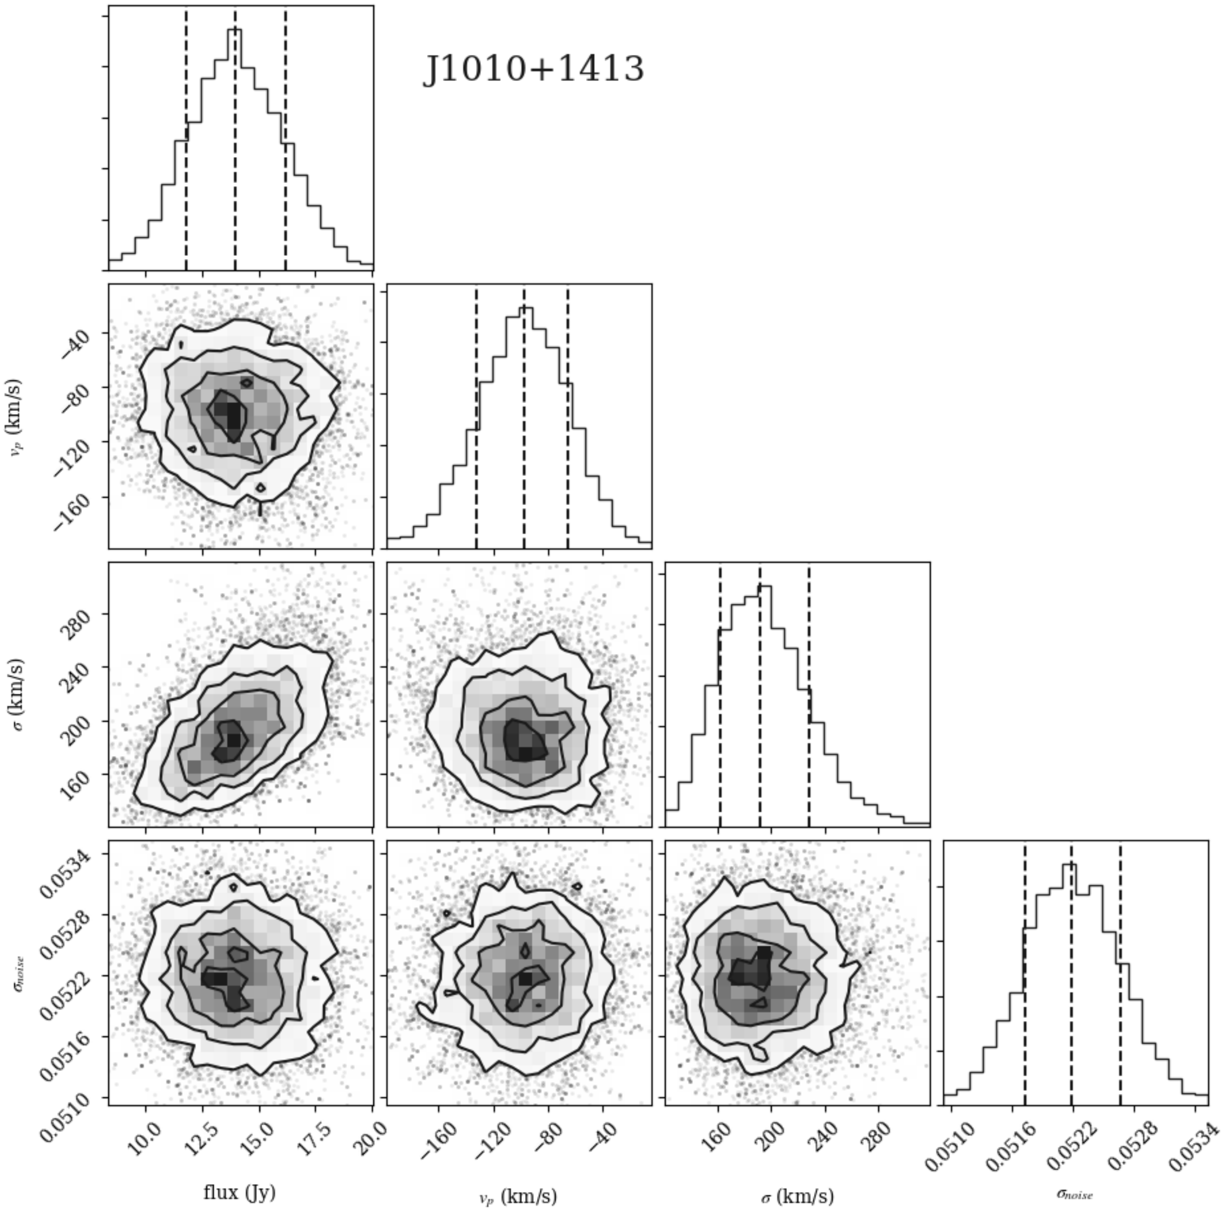


**Figure A4.** Same as Fig. A1 but for J1010+1413.

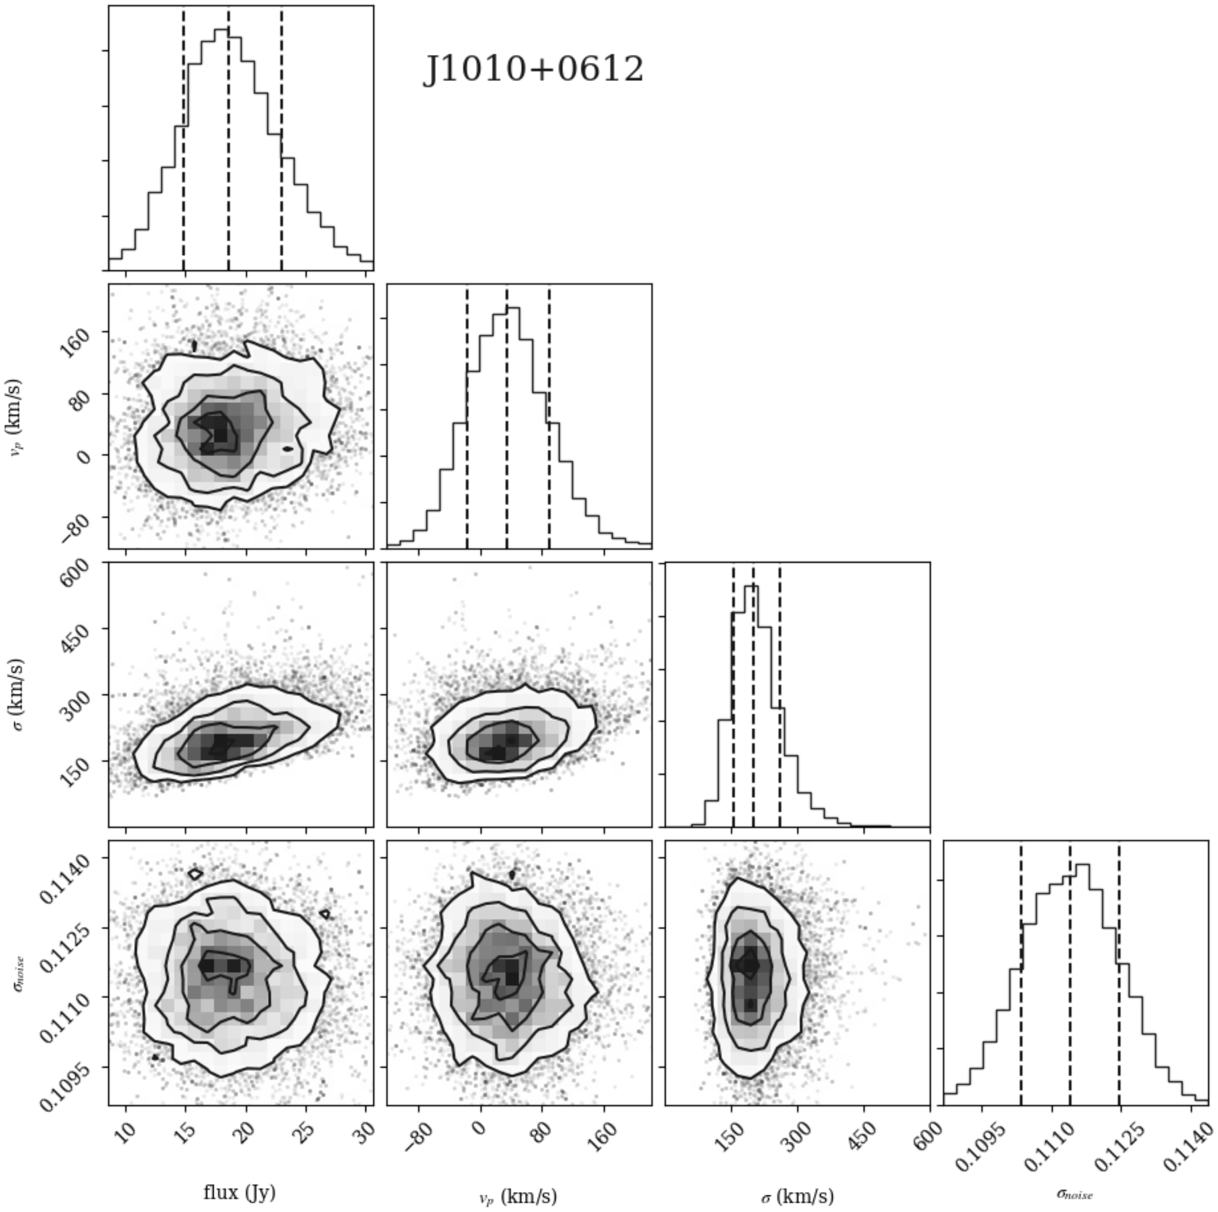


**Figure A5.** Same as Fig. A1 but for J1010+0612.

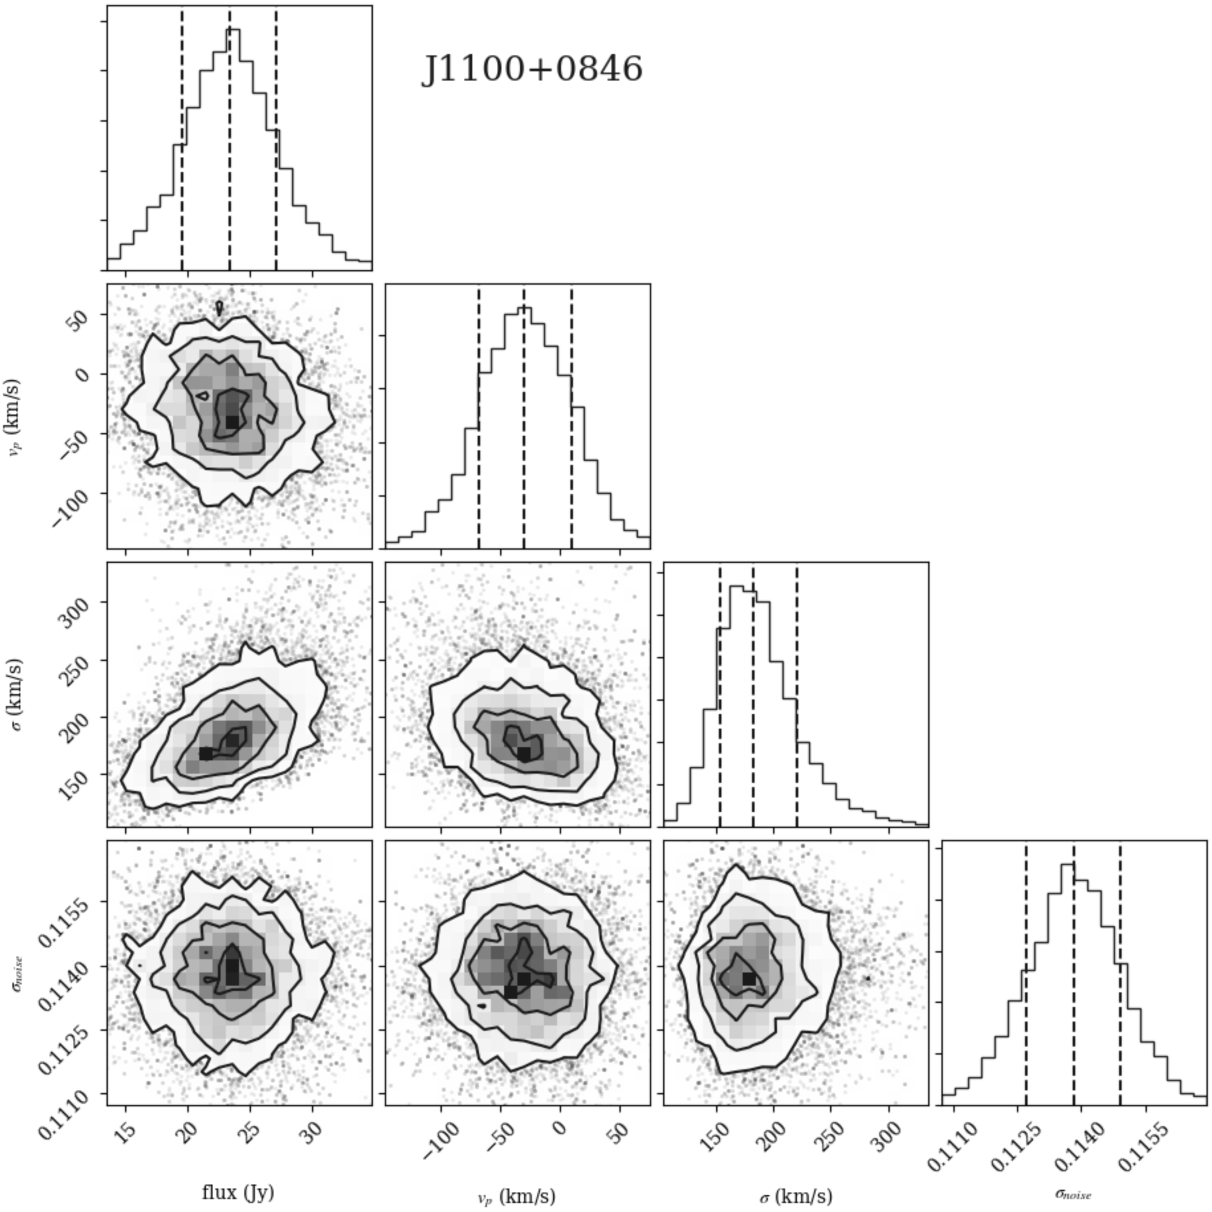


**Figure A6.** Same as Fig. A1 but for J1100+0846.

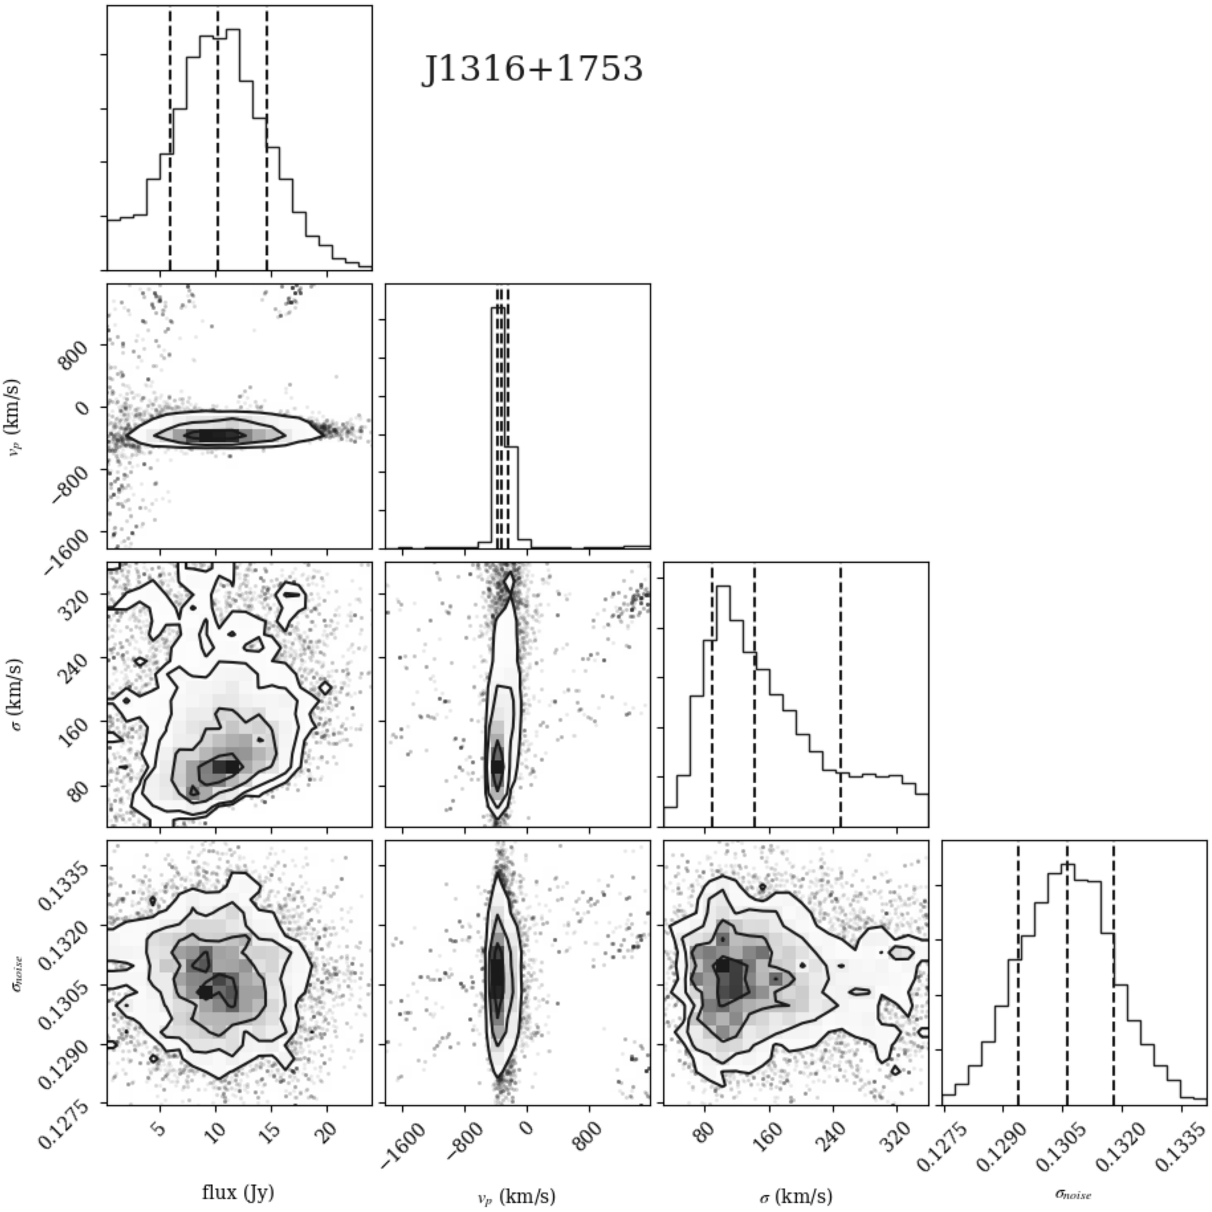


**Figure A7.** Same as Fig. A1 but for J1316+1753. Although we have a reliable measurement for the emission-line flux, we do not have as reliable constraints on the emission-line width; however, we do not use this value in this work.

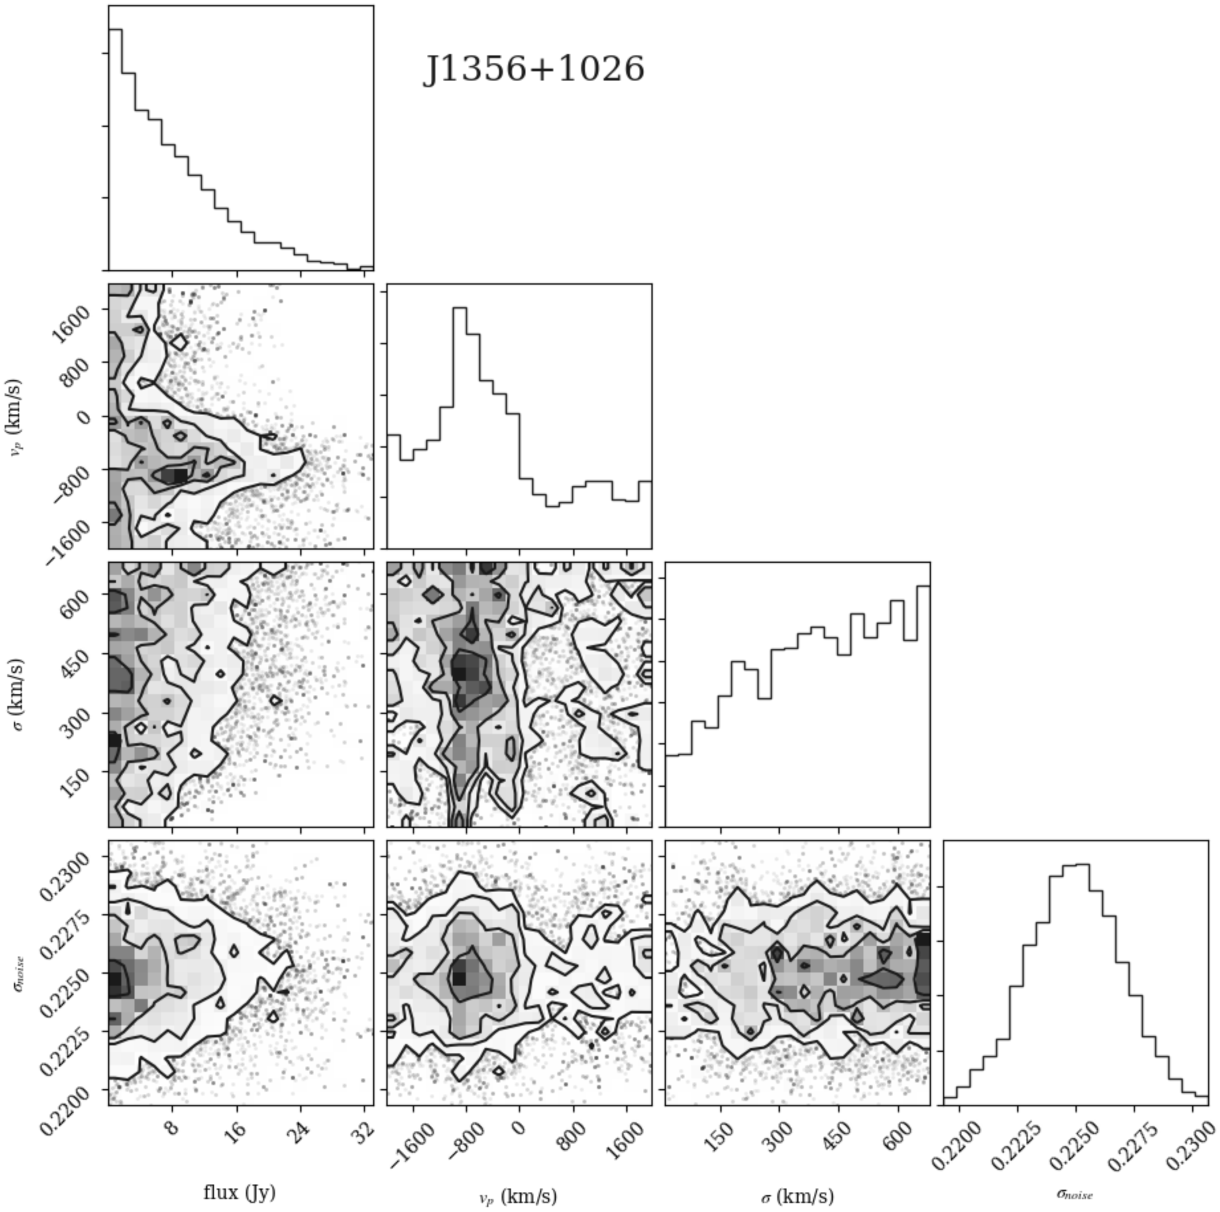


**Figure A8.** Same as Fig. A1 but for J1356+1026. The posteriors clearly show that the maximum allowed $\sigma$ is preferred, with the one dimensional posterior distribution for $\sigma$ rising steadily to the maximum value. Additionally the flux posterior peaks at zero. This support our identification of this data as a non-detection. The limit of the flux axes is the 99.7th percentile which is what we use as the upper limit of the CO(2–1) flux for our analysis.

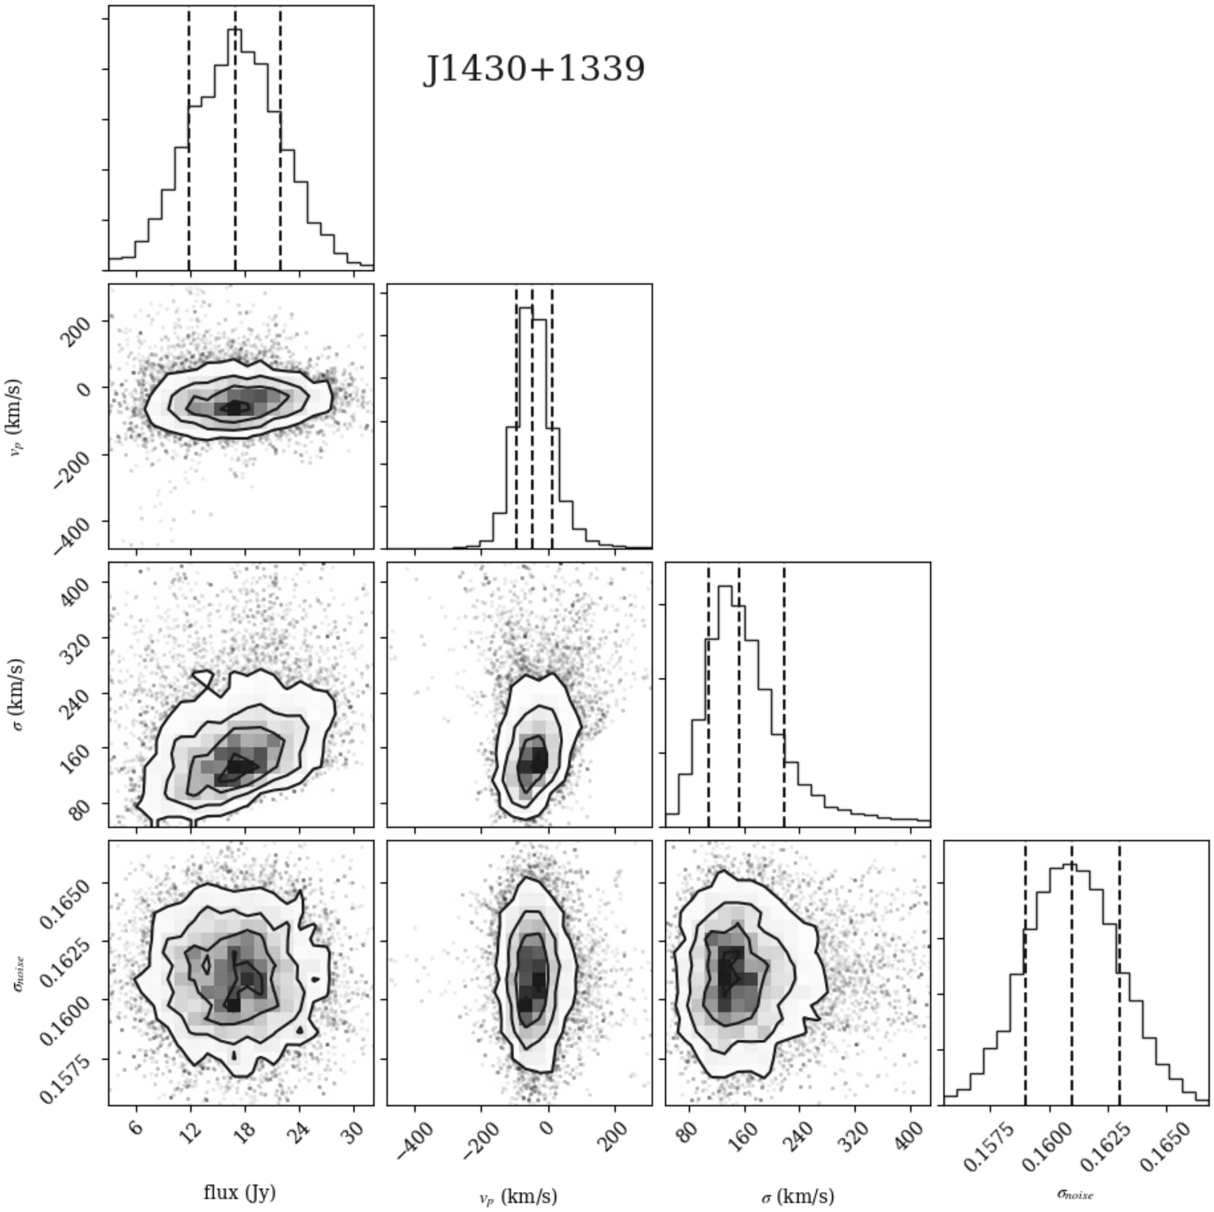


**Figure A9.** Same as Fig. A1 but for J1430+1339.

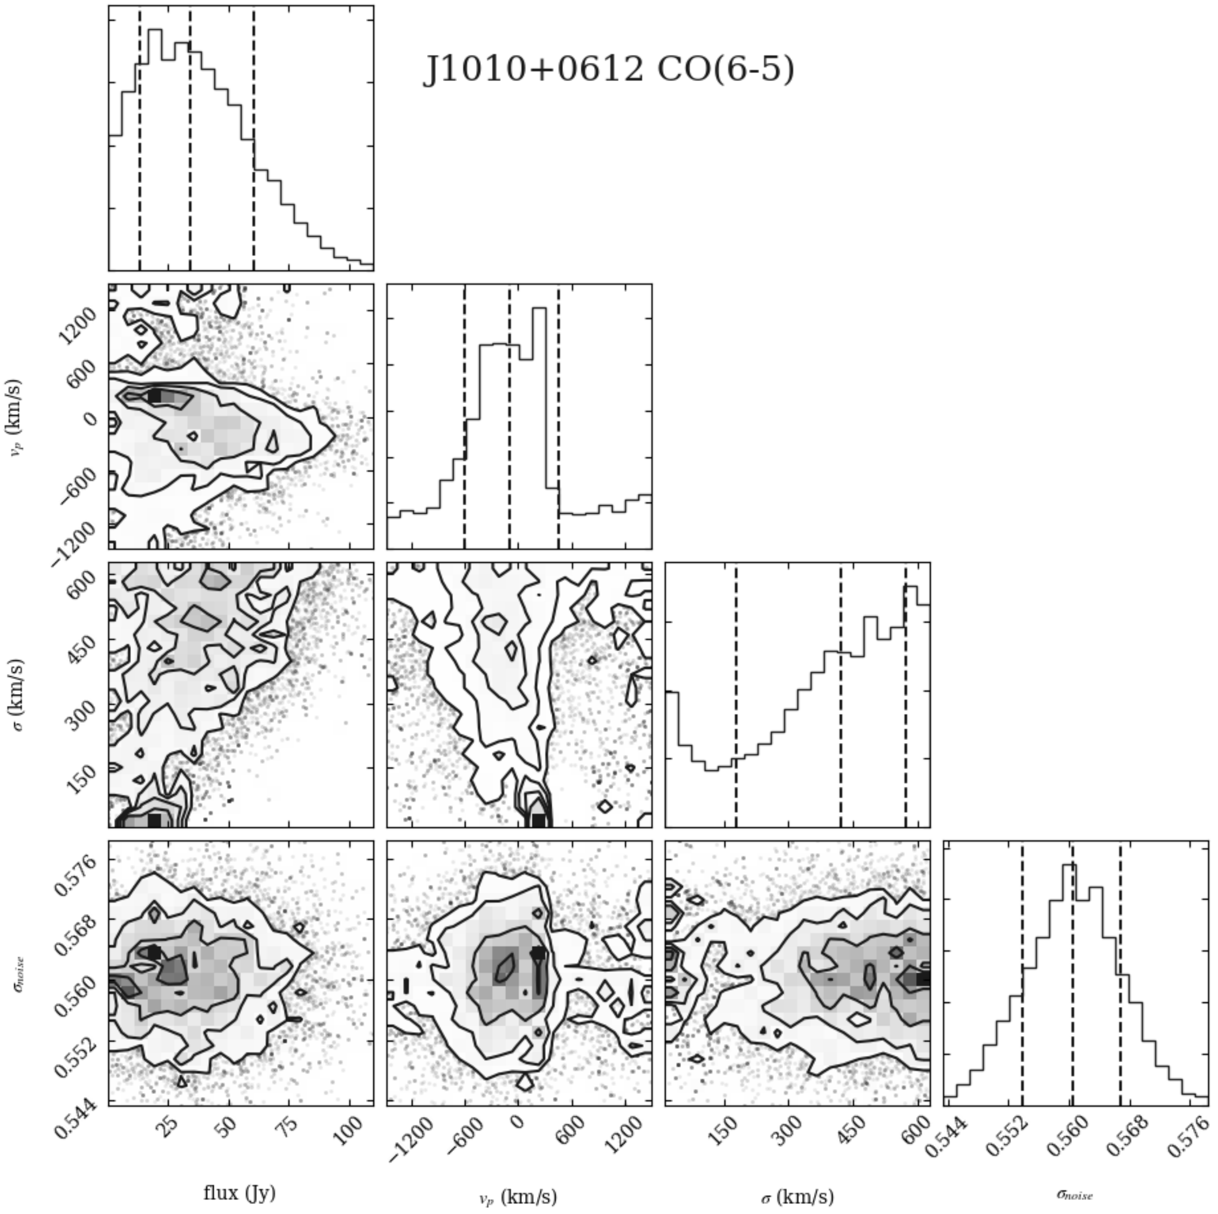


**Figure A10.** Same as Fig. A1 but for the APEX CO(6–5) data for J1010+0612. The posterior distribution for $\sigma$ in particular peaks at the highest possible value. This supports our identification of this data as a non-detection. The limit of the flux axes is the 99.7th percentile which is what we use as the upper limit of the CO(6–5) flux for our analysis.

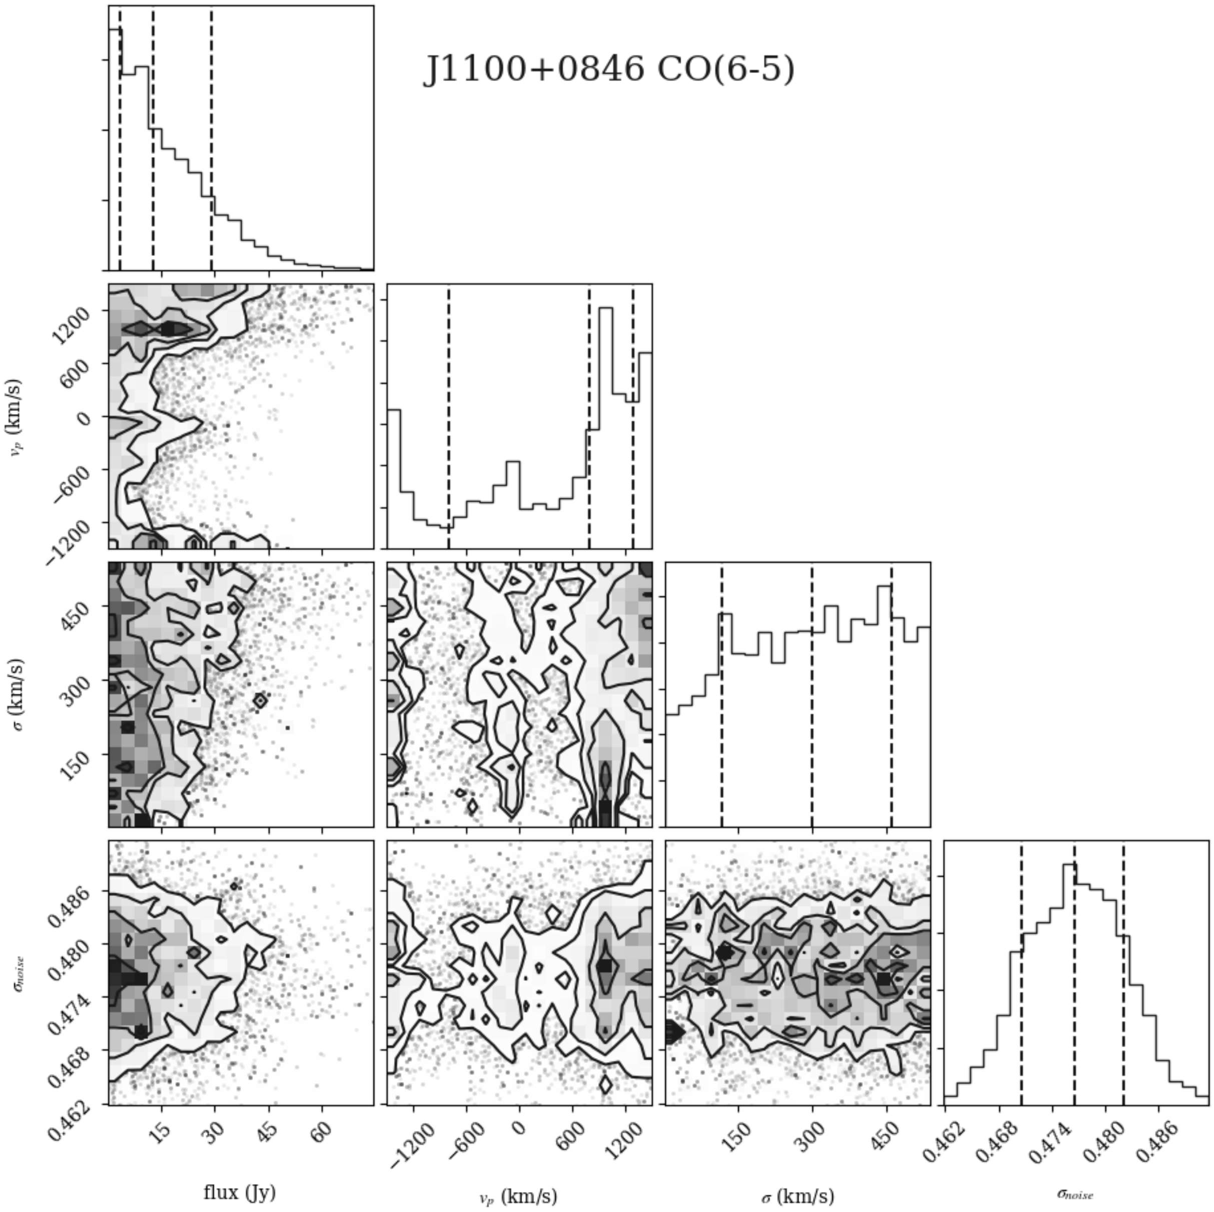


**Figure A11.** Same as Fig. A1 but for the APEX CO(6–5) data for J1100+0846. The posterior distribution for $\sigma$ in particular shows no clear peak, and the posterior distribution for the flux peaks at zero. This supports our identification of this data as a non-detection. The limit of the flux axes is the 99.7th percentile, which is what we use as the upper limit of the CO(6–5) flux for our analysis.

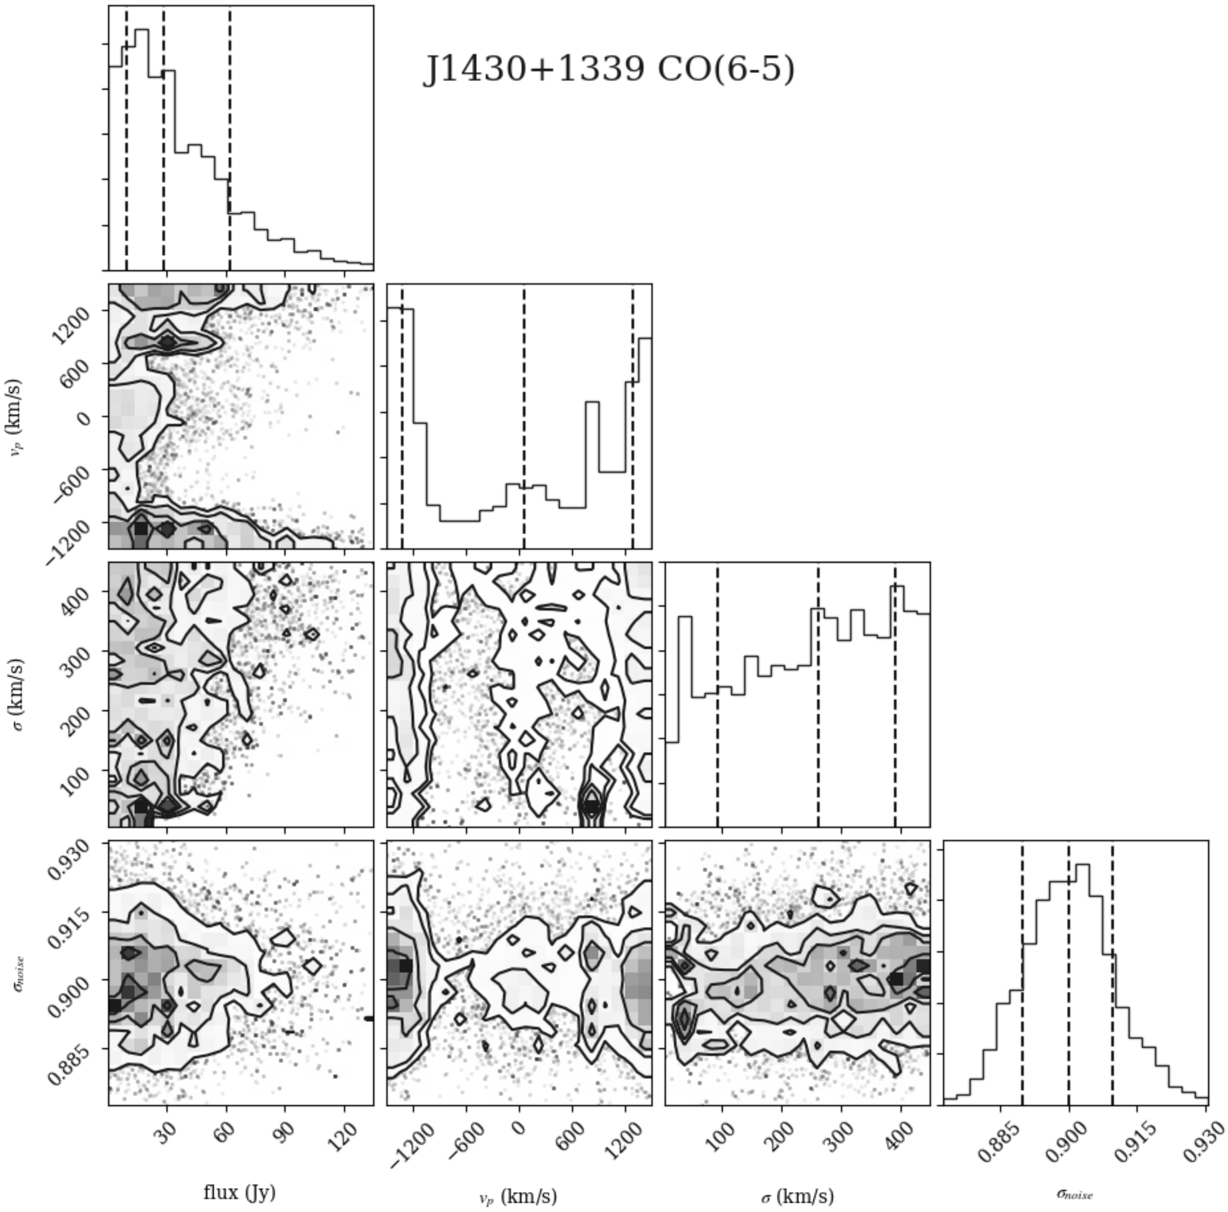


**Figure A12.** Same as Fig. A1 but for the APEX CO(6–5) data for J1430+1339. The posterior distribution for $\sigma$ in particular shows no clear peak, and the preferred $v_p$ values are at the edges, beyond where we would realistically expect the CO(6–5) line to lie. This supports our identification of this data as a non-detection. The limit of the flux axes is the 99.7th percentile which is what we use as the upper limit of the CO(6–5) flux for our analysis.
